# Supplementary material for: DCMT: A Direct Entire-Space Causal Multi-Task Framework for Post-Click Conversion Estimation
Source: arXiv:2302.06141 source file (2023-02-13)
Supplement: Supplementary file 1 [file appendix.tex]

\appendix
\section{APPENDIX}
\subsection{Task Definition}\label{Appendix_Task_Definition}
In this section, we define the three tasks, i.e., \emph{CTR Task}, \emph{CVR Task}, and \emph{CTCVR Task}, and formalize their probabilities respectively as follows.
\begin{myDef} \label{Definition_CTR}
 	\textbf{Click-Through Rate (CTR) Estimation}: Given a candidate exposure list of items, the goal of the CTR task is to predict the click-through probabilities of these items for a target user.
\end{myDef}
The above definition of the CTR prediction is to depict the probability of the behaviour path ``exposure$\rightarrow$click". For a target user $u_i$, the probability of post-exposure click-through of a candidate item $v_j$ can be represented as follows:
\begin{equation}\label{Equation_CTR}
	\begin{aligned}
	&\hat{o}_{i,j}=p(o_{i,j}=1|d_{i,j}=1,x_{i,j}),
	\end{aligned}
\end{equation}
where $x_{i,j }$ is the input features of a sample (the user-item pair $<u_i,v_j>$), $o_{i,j}$ is the click label of $u_i$ on item $v_j$ and $d_{i,j}$ is the exposure label of $v_j$ to user $u_i$, respectively.

\begin{myDef} \label{Definition_CVR}
 	\textbf{Conversion Rate (CVR) Estimation}: Given a candidate list of clicked items, the goal of the CVR task is to predict the conversion probabilities of these items for a target user.
\end{myDef}
The definition of CVR prediction is to depict the probability of the behaviour path ``click$\rightarrow$conversion". For a target user $u_i$, the probability of post-click conversion of a candidate item $v_j$ can be represented as follows:
\begin{equation}\label{Equation_CVR}
	\begin{aligned}
	&\hat{r}_{i,j}=p(r_{i,j}=1|o_{i,j}=1,x_{i,j}),
	\end{aligned}        
\end{equation}
where $r_{i,j}$ is the conversion label of $u_i$ on item $v_j$.

\begin{myDef} \label{Definition_CTCVR}
 	\textbf{Click-Through\&Conversion Rate (CTCVR) Estimation}: Given a candidate exposure list of items, the goal of the CTCVR task is to predict the click\&conversion probabilities of these items for a target user.
\end{myDef}
The corresponding probability can be represented as follows:
\begin{equation}\label{Equation_CTCVR}
	\begin{aligned}
	&\hat{t}_{i,j}=\hat{o}_{i,j}*\hat{r}_{i,j}.
	\end{aligned}        
\end{equation}

\subsection{The Theorems and Proofs for Unbiased CVR Estimation}\label{Appendix_proofs}
In this section, we provide the detailed theorems and proofs for the biased CVR estimation of ESMM and the unbiased CVR estimations of MTL-IPW, MTL-DR, and our DCMT as follows.

\begin{myTheorem}
The CVR estimation of ESMM is biased, i.e., Bias$^{\textrm{ESMM}}$ = $|E_{\mathcal{O}}(\mathcal{E}^{M}) - \mathcal{E}^{\textrm{ground-truth}}| > 0$
\end{myTheorem}
\begin{proof}
\begin{equation}\label{ESMM_is_biased}
	\begin{aligned}
&\textrm{Bias}^{\textrm{ESMM}} = \left| E_{\mathcal{O}}(\mathcal{E}^{\textrm{ESMM}}) - \mathcal{E}^{\textrm{ground-truth}} \right|\\
&=\bigg| \frac{1}{|\mathcal{D}|} \sum \limits_{(i,j) \in \mathcal{D}} (e_{i,j}^{\textrm{CTR}}+e_{i,j}^{\textrm{CTCVR}}) - \frac{1}{|\mathcal{D}|} \sum \limits_{(i,j) \in \mathcal{D}} e_{i,j}^{\textrm{CVR}}\bigg|\\
&=\frac{1}{|\mathcal{D}|} \bigg|\sum \limits_{(i,j) \in \mathcal{D}} (e_{i,j}^{\textrm{CTR}}+e_{i,j}^{\textrm{CTCVR}} - e_{i,j}^{\textrm{CVR}})\bigg|>0,
	\end{aligned}
\end{equation}
\end{proof}
where $e_{i,j}^{\textrm{CTR}} = e(o_{i,j},\hat{o}_{i,j})$, $e_{i,j}^{\textrm{CVR}} = e(r_{i,j},\hat{r}_{i,j})$, and $e_{i,j}^{\textrm{CTCVR}} = e(o_{i,j}*r_{i,j},\hat{o}_{i,j}*\hat{r}_{i,j})$. The authors in \cite{zhang2020large} have taken a toy example to verify that Bias$^{\textrm{ESMM}}>0$. Due to the space limitation, here, we directly quote their result.

\begin{myTheorem}
The CVR estimation of MTL-IPW is unbiased in the click space $\mathcal{O}$, i.e., Bias$^{\textrm{MTL-IPW}}$ = $|E_{\mathcal{O}}(\mathcal{E}^{\textrm{MTL-IPW}}) - \mathcal{E}^{\textrm{ground-truth}}| = 0$, when $o_{i,j}=\hat{o}_{i,j}$, i.e., the prediction of click propensity is accurate.
\end{myTheorem}
\begin{proof}
\begin{equation}\label{Unbiased_Proof}
	\begin{aligned}
&\textrm{Bias}^{\textrm{MTL-IPW}} = \left| E_{\mathcal{O}}(\mathcal{E}^{\textrm{MTL-IPW}}) - \mathcal{E}^{\textrm{ground-truth}} \right|\\
&=\bigg| \frac{1}{|\mathcal{D}|} \sum \limits_{(i,j) \in \mathcal{D}} \frac{o_{i,j}e(r_{i,j},\hat{r}_{i,j})}{\hat{o}_{i,j}} - \frac{1}{|\mathcal{D}|} \sum \limits_{(i,j) \in \mathcal{D}} e(r_{i,j},\hat{r}_{i,j})\bigg|\\
&=\frac{1}{|\mathcal{D}|} \bigg|\sum \limits_{(i,j) \in \mathcal{D}} (\frac{o_{i,j}}{\hat{o}_{i,j}} - 1) e(r_{i,j},\hat{r}_{i,j})\bigg|=0.
	\end{aligned}
\end{equation}
\end{proof}

\begin{myTheorem}
The CVR estimation of MTL-DR is unbiased in the exposure space $\mathcal{D}$, i.e., Bias$^{\textrm{MTL-DR}}$ = $|E_{\mathcal{O}}(\mathcal{E}^{\textrm{MTL-DR}}) - \mathcal{E}^{\textrm{ground-truth}}| = 0$, when $o_{i,j}=\hat{o}_{i,j}$ or $\delta_{i,j}=e_{i,j}-\hat{e}_{i,j}=0$, i.e., the prediction of click propensity is accurate or the prediction of CVR error is accurate.
\end{myTheorem}
\begin{proof}
\begin{equation}\label{Unbiased_Proof_DR}
	\begin{aligned}
&\textrm{Bias}^{\textrm{MTL-DR}} = \left| E_{\mathcal{O}}(\mathcal{E}^{\textrm{MTL-DR}}) - \mathcal{E}^{\textrm{ground-truth}} \right|\\
&=\bigg| \frac{1}{|\mathcal{D}|} \sum \limits_{(i,j) \in \mathcal{D}} \big( \hat{e}_{i,j} + \frac{o_{i,j}\delta_{i,j}}{\hat{o}_{i,j}}\big) - \frac{1}{|\mathcal{D}|} \sum \limits_{(i,j) \in \mathcal{D}} e_{i,j}\bigg|\\
&=\frac{1}{|\mathcal{D}|} \bigg|\sum \limits_{(i,j) \in \mathcal{D}} \frac{\hat{e}_{i,j}\hat{o}_{i,j}+o_{i,j}\delta_{i,j}-\hat{o}_{i,j}e_{i,j}}{\hat{o}_{i,j}}\bigg|\\
&=\frac{1}{|\mathcal{D}|} \bigg|\sum \limits_{(i,j) \in \mathcal{D}} \frac{(o_{i,j}-\hat{o}_{i,j})\delta_{i,j}}{\hat{o}_{i,j}}\bigg| =0.
	\end{aligned}
\end{equation}
\end{proof}

\begin{myTheorem}
The CVR estimation of our DCMT is unbiased in the exposure space $\mathcal{D}$, i.e., Bias$^{\textrm{DCMT}}$ = $|E_{\mathcal{O}}(\mathcal{E}^{\textrm{DCMT}}) - \mathcal{E}^{\textrm{ground-truth}}| = 0$, when $o_{i,j}=\hat{o}_{i,j}$ and $\hat{r}_{i,j}+\hat{r}^*_{i,j}=1$, i.e., the prediction of click propensity is accurate and the predictions of factual CVR and counterfactual CVR follow the counterfactual prior knowledge.
\end{myTheorem}

Note that $o_{i,j}=\hat{o}_{i,j}$ means that $o_{i,j}=\hat{o}_{i,j}=1$ in the click space $\mathcal{O}$ and $o_{i,j}=\hat{o}_{i,j}=0$ in the non-click space $\mathcal{N}$. Meanwhile, $\hat{r}_{i,j}+\hat{r}^*_{i,j}=1$ means that the counterfactual regularizer $L=0$ and  $e(1-r_{i,j},\hat{r}^*_{i,j})=e(1-r_{i,j},1-\hat{r}_{i,j})=e(r_{i,j},\hat{r}_{i,j})$ because $e(r_{i,j},\hat{r}_{i,j})$ is the log loss.

\begin{proof}
\begin{equation}\label{DCMT_bias}
	\begin{aligned}
&\textrm{Bias}^{\textrm{DCMT}} = \left| \mathcal{E}^{\textrm{DCMT}} - \mathcal{E}^{\textrm{ground-truth}} \right|\\
=&\bigg| \frac{1}{|\mathcal{D}|} \bigg( \sum \limits_{(i,j) \in \mathcal{O}} \frac{e(r_{i,j},\hat{r}_{i,j})}{\hat{o}_{i,j}} + \sum \limits_{(i,j) \in \mathcal{N^*}} \frac{e(r^*_{i,j},\hat{r}^*_{i,j})}{1-\hat{o}_{i,j}}\bigg)\\
	&+ L - \frac{1}{|\mathcal{D}|} \sum \limits_{(i,j) \in \mathcal{D}} e(r_{i,j},\hat{r}_{i,j})\bigg|\\
=&\bigg|\frac{1}{|\mathcal{D}|} \bigg( \sum \limits_{(i,j) \in \mathcal{O}} \frac{e(r_{i,j},\hat{r}_{i,j})}{\hat{o}_{i,j}} + \sum \limits_{(i,j) \in \mathcal{N}} \frac{e(1-r_{i,j},\hat{r}^*_{i,j})}{1-\hat{o}_{i,j}}\bigg)+ L\\
	& - \frac{1}{|\mathcal{D}|} \sum \limits_{(i,j) \in \mathcal{D}} e(r_{i,j},\hat{r}_{i,j})\bigg|\\
=&\bigg| \frac{1}{|\mathcal{D}|} \sum \limits_{(i,j) \in \mathcal{O}} \frac{(1-\hat{o}_{i,j})e(r_{i,j},\hat{r}_{i,j})}{\hat{o}_{i,j}} + L\\
&+ \frac{1}{|\mathcal{D}|}\sum \limits_{(i,j) \in \mathcal{N}} \frac{e(1-r_{i,j},\hat{r}^*_{i,j}) - (1-\hat{o}_{i,j})e(r_{i,j},\hat{r}_{i,j})}{1-\hat{o}_{i,j}}\bigg|=0\\
	\end{aligned}
\end{equation}
\end{proof}

\subsection{Embedding Layer} \label{Appendix_Details_of_Embedding_Layer}
As introduced in Section \ref{Section_overview}, we have classified the sparse ID features, dense numerical features, and weighted features, of users, items, and user-item interactions, into two categories, i.e., deep features and wide features. Therefore, we can generate the concatenated deep embeddings and the concatenated wide embeddings (see \emph{Embedding Layer} in Fig. \ref{our_model_structure}), respectively. Next, we will explain the details of feature embedding generation in the following section.

\subsubsection{Feature Embedding Generation}\label{feature_embedding_generation}
It is worth noting that the existing embedding strategies for post-click conversion prediction are missing or confused in many existing approaches. Therefore, in this paper, we design the strategies of embedding generation for three main types of features as follows.

\nosection{Sparse ID Features} As for sparse ID features, we first convert them to identity values, and then convert them to a dense representation by feeding them to a fully-connected neural network.

\nosection{Dense Numerical Features} As for dense numerical features, we first concatenate all dense numerical features in the same group and feed them to a fully-connected neural network. The output of the neural network is the embedding of these dense features.

\nosection{Weighted Features} There are some weighted features in real applications, e.g., the user historical behaviours of shop ID and weights in the Ali-CCP dataset. According to the above two embedding strategies, we can first obtain the embeddings of Sparse IDs and then we adopt average-pooling to generate the mean of weighted embeddings.
